# Supplementary material for: Bifurcation Analysis of Reaction Diffusion Systems on Arbitrary Surfaces
Source: arXiv:1605.01583 ancillary file (2016-05-05)
Supplement: Supplementary file 1 [file SM01.pdf]

# Bifurcation Analysis of Reaction Diffusion Systems on Arbitrary Surfaces
# SM01: Detailed Mathematical Derivations

## D1 Reaction Diffusion System Coefficients upon Linearisation

A two-component general RD system with cross diffusion is expressed mathematically as

$$\begin{aligned}\frac{\partial a}{\partial t} &= \nabla^2\left[\left({}^aD_a + {}^aD_\alpha a + {}^aD_\beta b\right)a\right] + f(a,b),\\ \frac{\partial b}{\partial t} &= \nabla^2\left[\left({}^bD_b + {}^bD_\alpha a + {}^bD_\beta b\right)b\right] + g(a,b).\end{aligned} \tag{1}$$

Refer to Section 3.1 in the main paper for details about the terms involved. Now, near a given steady state $(a_0, b_0)$, we substitute $a = a_0 + u$ and $b = b_0 + v$ in Equation 1 with $u = \Delta a|_{a_0}$ and $v = \Delta b|_{b_0}$ as infinitesimal deviations. This give us,

$$\frac{\partial(a_0+u)}{\partial t} = \nabla^2\left[\left({}^aD_a + {}^aD_\alpha(a_0+u) + {}^aD_\beta(b_0+v)\right)(a_0+u)\right] + f(a_0+u, b_0+v).$$

Upon expansion, we get

$$\begin{aligned}\frac{\partial a_0}{\partial t} + \frac{\partial u}{\partial t} =& \nabla^2\left[\left({}^aD_a + {}^aD_\alpha a_0 + {}^aD_\beta b_0\right)a_0\right] + \nabla^2\left[\left({}^aD_a + {}^aD_\alpha a_0 + {}^aD_\beta b_0\right)u\right] +\\ &\nabla^2\left[\left({}^aD_\alpha u + {}^aD_\beta v\right)(a_0+u)\right] + f(a_0+u, b_0+v).\end{aligned} \tag{2}$$

Substituting $f(a_0+u, b_0+v)$ from Equation 2 in the main paper into Equation 2 here results in

$$\begin{aligned}\frac{\partial a_0}{\partial t} + \frac{\partial u}{\partial t} =& \nabla^2\left[\left({}^aD_a + {}^aD_\alpha a_0 + {}^aD_\beta b_0\right)a_0\right] + \nabla^2\left[\left({}^aD_a + {}^aD_\alpha a_0 + {}^aD_\beta b_0\right)u\right] +\\ &\nabla^2\left[\left({}^aD_\alpha u + {}^aD_\beta v\right)(a_0+u)\right] + f(a_0,b_0) +\\ &u\left.\frac{\partial f}{\partial a}\right|_{(a_0,b_0)} + v\left.\frac{\partial f}{\partial b}\right|_{(a_0,b_0)} + n_f(u,v),\end{aligned} \tag{3}$$

where, $n_f(u,v)$ contains second and higher order terms in $u$ and $v$ for the Taylor series expansion of $f(a,b)$ at $a = a_0 + u$ and $b = b_0 + v$. Now $(a_0, b_0)$ is a steady

state solution for Equation 1 and thus we have

$$\frac{\partial a_0}{\partial t} = \nabla^2 \left[ \left( {}^aD_a + {}^aD_\alpha a_0 + {}^aD_\beta b_0 \right) a_0 \right] + f(a_0, b_0).$$

Substituting this in Equation 3 yields,

$$\begin{aligned}
\frac{\partial u}{\partial t} &= \nabla^2 \left[ \left( {}^aD_a + {}^aD_\alpha a_0 + {}^aD_\beta b_0 \right) u \right] + \nabla^2 \left[ \left( {}^aD_\alpha u + {}^aD_\beta v \right) (a_0 + u) \right] + \\
&\qquad u \left. \frac{\partial f}{\partial a} \right|_{(a_0,b_0)} + v \left. \frac{\partial f}{\partial b} \right|_{(a_0,b_0)} + n_f(u,v) \\
&= \left( {}^aD_a + 2\,{}^aD_\alpha a_0 + {}^aD_\beta b_0 \right) \nabla^2 u + {}^aD_\beta a_0 \nabla^2 v + u \left. \frac{\partial f}{\partial a} \right|_{(a_0,b_0)} + v \left. \frac{\partial f}{\partial b} \right|_{(a_0,b_0)} + \\
&\qquad {}^aD_\alpha \nabla^2 u^2 + {}^aD_\beta \nabla^2 uv + n_f(u,v) \qquad (4)
\end{aligned}$$

Now since $|u| \ll a_0$ and $|v| \ll b_0$ near homogeneity, the second and higher order terms in $u, v$ are negligible and we can ignore them. Also, substituting

$$\begin{aligned}
&{}^uD_u = {}^aD_a + 2\,{}^aD_\alpha a_0 + {}^aD_\beta b_0, \quad {}^uD_v = {}^aD_\beta a_0, \quad {}^uK_u = \left. \frac{\partial f}{\partial a} \right|_{(a_0,b_0)}, \text{ and} \\
&{}^uK_v = \left. \frac{\partial f}{\partial b} \right|_{(a_0,b_0)} \qquad (5)
\end{aligned}$$

in Equation 4 results in,

$$\frac{\partial u}{\partial t} = {}^uD_u \nabla^2 u + {}^uD_v \nabla^2 v + {}^uK_u u + {}^uK_v v. \qquad (6)$$

Similarly, we can derive

$$\frac{\partial v}{\partial t} = {}^vD_v \nabla^2 v + {}^vD_u \nabla^2 u + {}^vK_u u + {}^vK_v v, \qquad (7)$$

with

$$\begin{aligned}
&{}^vD_v = {}^bD_b + 2\,{}^bD_\beta b_0 + {}^bD_\alpha a_0, \quad {}^vD_u = {}^bD_\alpha b_0, \quad {}^vK_v = \left. \frac{\partial g}{\partial b} \right|_{(a_0,b_0)}, \text{ and} \\
&{}^vK_u = \left. \frac{\partial g}{\partial a} \right|_{(a_0,b_0)} \qquad (8)
\end{aligned}$$

Equations 6 and 7 express the same linearised RD system as Equation 3 in the main paper. Also Equations 5 and 8 define new diffusion coefficients $\{{}^uD_u, {}^uD_v, {}^vD_u, {}^vD_v\}$ and reaction coefficients $\{{}^uK_u, {}^uK_v, {}^vK_u, {}^vK_v\}$ for the RD system linearised at $(a_0, b_0)$.

## D2 Boundary Conditions satisfying the *Hermitian* property for the *Laplace-Beltrami* operator

Consider the Laplace-Beltrami operator $L \equiv \nabla^2$ operating on a set $S_f$ of smooth real-valued functions such as $u$ and $v$ which are defined over an arbitrary surface $\Omega \subset \mathbf{R}^3$. For $L$ to be Hermitian, it must satisfy $\langle u, Lv \rangle = \langle Lu, v \rangle$, where $\langle ., . \rangle$ defines an *inner product* of functions $x$ and $y$ as $\langle x, y \rangle = \int_\Omega xy \, \mathrm{d}\Omega$. Now consider the equality of $\langle u, Lv \rangle$ and $\langle Lu, v \rangle$, i.e.,

$$\int_\Omega u \nabla^2 v \, \mathrm{d}\Omega \quad \stackrel{?}{=} \quad \int_\Omega v \nabla^2 u \, \mathrm{d}\Omega \, .$$

Using *Green's first identity** on both sides to perform integration-by-parts we get,

$$-\int_\Omega \nabla u \cdot \nabla v \, \mathrm{d}\Omega + \oint_\Gamma u(\nabla v \cdot \widehat{n}) \mathrm{d}\Gamma \quad \stackrel{?}{=} \quad -\int_\Omega \nabla u \cdot \nabla v \, \mathrm{d}\Omega \quad + \oint_\Gamma v(\nabla u \cdot \widehat{n}) \mathrm{d}\Gamma,$$

$$\text{i.e.} \quad \oint_\Gamma u(\nabla v \cdot \widehat{n}) \mathrm{d}\Gamma \quad \stackrel{?}{=} \quad \oint_\Gamma v(\nabla u \cdot \widehat{n}) \mathrm{d}\Gamma \, . \tag{9}$$

Here, $\nabla u$ and $\nabla v$ are the surface gradients for $u$ and $v$ respectively, $\Gamma$ is the smooth boundary for $\Omega$ and $\widehat{n}$ is the outward pointing surface normal of the boundary surface element $\mathrm{d}\Gamma$. Clearly, if Equation 9 is satisfied by every pair of surface function $u, v \in S_f$, then the Laplace-Beltrami operator $\nabla^2$ is Hermitian and it can be used to generate a set of orthonormal basis functions for all functions $f \in S_f$ defined over the domain $\Omega$. Next, we consider common boundary conditions imposed on biological systems (i.e. on $S_f$) and show how they satisfy the Hermitian property of the Laplace-Beltrami operator $\nabla^2$.

**Case (0) : A surface with no boundaries.** For surfaces with no boundaries, the boundary integral terms in Equation 9 do not exist and thus $\langle u, Lv \rangle = \langle Lu, v \rangle$, $\forall u, v \in S_f$.

**Case (i) : Zero Robin boundary conditions.** For zero Robin boundary conditions, at boundary $\Gamma$ , $cu + d(\nabla u \cdot \widehat{n}) = cv + d(\nabla v \cdot \widehat{n}) = 0$ for some arbitrary smooth functions $c$ and $d$ defined over the surface boundary $\Gamma$. Thus Equation 9 becomes,

$$\oint_\Gamma u(\frac{-cv}{d}) \mathrm{d}\Gamma \stackrel{?}{=} \oint_\Gamma v(\frac{-cu}{d}) \mathrm{d}\Gamma \, .$$

It is self-evident that above equation holds true for nonzero functions $d$.

*We assume that the surface function is extended in an infinitesimally small region around the surface such that its surface derivatives equal the spatial derivatives of the extended function.

**Case (ii) : Zero Dirichlet boundary conditions.** Note that Dirichlet boundary conditions are a special case of Robin boundary conditions with $c = 1$ and $d = 0$. However, since $d = 0$, we fall-back to Equation 9 for this case. With, zero Dirichlet boundary conditions, $u = v = 0$ at boundary $\Gamma$. Thus,

$$\oint_{\Gamma} u(\nabla v \cdot \widehat{n}) \mathrm{d}\Gamma \;=\; \oint_{\Gamma} v(\nabla u \cdot \widehat{n}) \mathrm{d}\Gamma = 0 \,.$$

**Case (iii) : Zero Neumann boundary conditions.** Again, Neumann boundary conditions are a special case of Robin boundary conditions with $c = 0$ and $d = 1$. Thus, for zero Neumann boundary conditions, since $d$ is non-zero, the Hermitian property are satisfied as in the case of Robin boundary conditions.

**Case (iv) : Periodic boundary conditions.** In biological systems, periodic boundary conditions are generally used to replicate the conditions for closed surfaces as in case (0) while simulating only a small part of it. Nevertheless, we show mathematically how, in general, periodic boundary conditions satisfy the *Hermitian* property for the Laplace-Beltrami operator. To do this, let us represent domain $\Omega$ parametrically with $r_1$ and $r_2$, without any loss of generality. Thus for our smooth functions $u$ and $v$ we express fundamental periodicities $R_1$ and $R_2$ with equations: $u(r_1, r_2) = u(r_1 + R_1, r_2 + R_2)$ and $v(r_1, r_2) = v(r_1 + R_1, r_2 + R_2)$. The figure above shows four boundary segments $\Gamma_1$, $\Gamma_2$, $\Gamma_3$ and $\Gamma_4$ representing periodic boundary conditions. Now, by substituting these boundaries and periodicities in the L.H.S for Equation 9 we get,

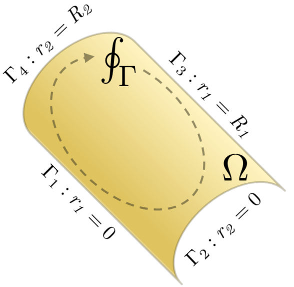


$$L.H.S. = \oint_{\Gamma} u(\nabla v \cdot \widehat{n}) \mathrm{d}\Gamma \quad = \oint_{\Gamma_1+\Gamma_2+\Gamma_3+\Gamma_4} u(\nabla v \cdot \widehat{n}) \mathrm{d}\Gamma = \quad I_1 + I_2 \quad (\text{say}) \,.$$

Here, $I_1$ represents integration over $\Gamma_1 + \Gamma_3$ and $I_2$ over $\Gamma_2 + \Gamma_4$. Thus,

$$\begin{aligned} I_1 &= \oint_{0}^{R_2} u(0, r_2)(\nabla v(0, r_2) \cdot \widehat{n}(0, r_2)) \mathrm{d}r_2 + \oint_{R_2}^{0} u(R_1, r_2)(\nabla v(R_1, r_2) \cdot \widehat{n}(R_1, r_2)) \mathrm{d}r_2 , \\ &= \oint_{0}^{R_2} u(0, r_2)(\nabla v(0, r_2) \cdot \widehat{n}(0, r_2)) \mathrm{d}r_2 + \oint_{R_2}^{0} u(0, r_2)(\nabla v(0, r_2) \cdot \widehat{n}(0, r_2)) \mathrm{d}r_2 , \\ &= 0 \,. \end{aligned}$$

Similarly, $I_2 = 0$ and also $R.H.S. = 0$. Thus $\langle u, Lv \rangle = \langle Lu, v \rangle$, $\forall x, y \in S_f$ with periodic boundary conditions. In conclusion, all boundary conditions discussed above result in a *Hermitian* linear Laplace-Beltrami operator $\nabla^2$.

## D3 Relation between the Spectral Coefficients and the Eigenvalues

From Equation 7 in the main paper, we have

$$
\begin{aligned}
& {}^{u}D_u \nabla^2 \sum_k u_k \phi_k + {}^{u}D_v \nabla^2 \sum_k v_k \phi_k + {}^{u}K_u \sum_k u_k \phi_k + {}^{u}K_v \sum_k v_k \phi_k = 0, \\
\text{i.e.}\quad & {}^{u}D_u \sum_k u_k \nabla^2 \phi_k + {}^{u}D_v \sum_k v_k \nabla^2 \phi_k + {}^{u}K_u \sum_k u_k \phi_k + {}^{u}K_v \sum_k v_k \phi_k = 0.
\end{aligned}
$$

Please refer to the main paper for details of the terms involved. Since each $\phi_k$ is an eigenfunction of the Laplace-Beltrami operator $\nabla^2$ with an eigenvalue $\lambda_k$, we have $\nabla^2 \phi_k = -\lambda_k \phi_k$. Substituting this in the above equation gives us

$$
\begin{aligned}
& -{}^{u}D_u \sum_k u_k \lambda_k \phi_k - {}^{u}D_v \sum_k v_k \lambda_k \phi_k + {}^{u}K_u \sum_k u_k \phi_k + {}^{u}K_v \sum_k v_k \phi_k = 0, \\
\text{i.e.}\quad & \sum_k \left({}^{u}K_u - {}^{u}D_u \lambda_k\right) u_k \phi_k + \sum_k \left({}^{u}K_v - {}^{u}D_v \lambda_k\right) v_k \phi_k = 0.
\end{aligned}
$$

Now, multiplying both sides of the equation above with an eigenfunction $\phi_j$ and integrating over the surface domain $\Omega$ results in

$$
\begin{aligned}
& \int_\Omega \left( \sum_k \left({}^{u}K_u - {}^{u}D_u \lambda_k\right) u_k \phi_k \right) \phi_j + \int_\Omega \left( \sum_k \left({}^{u}K_v - {}^{u}D_v \lambda_k\right) v_k \phi_k \right) \phi_j = 0. \\
\text{i.e.}\quad & \sum_k \left( \left({}^{u}K_u - {}^{u}D_u \lambda_k\right) u_k \int_\Omega \phi_k \phi_j \right) + \sum_k \left( \left({}^{u}K_v - {}^{u}D_v \lambda_k\right) v_k \int_\Omega \phi_k \phi_j \right) = 0.
\end{aligned}
$$

For the boundary conditions discussed in Section D2, the LB operator $\nabla^2$ is *Hermitian* and the eigenfunctions such as $\phi_k$ and $\phi_j$ form an orthonormal basis set. In other words, $\int_\Omega \phi_k \phi_j = 1$, if $j = k$, else $\int_\Omega \phi_k \phi_j = 0$. Substituting these integral values in the equation above yields

$$
\left({}^{u}K_u - {}^{u}D_u \lambda_k\right) u_k + \left({}^{u}K_v - {}^{u}D_v \lambda_k\right) v_k = 0, \quad \forall k. \tag{10}
$$

Similarly, by expanding the second part of Equation 7 and subjecting it to a *weak formulation Galerkin* integration, as above, we can show that

$$
\left({}^{v}K_v - {}^{v}D_v \lambda_k\right) v_k + \left({}^{v}K_u - {}^{v}D_u \lambda_k\right) u_k = 0, \quad \forall k. \tag{11}
$$

Equations 10 and 11 express the relation between the spectral coefficients $u_k$ and $v_k$ and the eigenvalues $\lambda_k$ as given in Equation 8 in the main paper.

## D4 Reaction Coefficients for Mixed-mode Bifurcations

Here, we derive the formulae for reaction coefficients of a linearised RD system at a mixed-mode bifurcation. As discussed in Section 3.4.3, two sets of eigenmodes, $\{\phi_i \,|\, \lambda_i = \Lambda_m\}$ and $\{\phi_j \,|\, \lambda_j = \Lambda_n\}$, participate in formation of an emergent pattern. Here $\Lambda_m$ and $\Lambda_n$ are the eigenvalues that satisfy Equations 10 and 11 for all spectral coefficient pairs $< u_i, v_i >$ and $< u_j, v_j >$ respectively. Again, as in Section 3.4.3 (Main Paper), we define $s_i = v_i/u_i$. For a given eigenmode $\phi_i$, by substituting $\lambda_k = \Lambda_m$, $u_k = u_i$ and $v_k = v_i = s_i u_i$ in Equation 10 we get,

$$({}^uK_u - {}^uD_u\Lambda_m)\,u_i \;+\; ({}^uK_v - {}^uD_v\Lambda_m)\,s_i u_i \;=\; 0, \quad \text{i.e.} \quad s_i = \frac{{}^uK_u - {}^uD_u\Lambda_m}{{}^uK_v - {}^uD_v\Lambda_m}. \quad (12)$$

The above derivation assumes that $u_i \neq 0$, which is true since we only consider those eigenmodes that contribute to the emergent pattern. Since all system parameters are fixed at a bifurcation point, Equation 12 implies that $s_i$ can have only one value $\forall i$ at a given bifurcation point. Similarly, $s_j$ can have only one value $\forall j$ at a given bifurcation point. We denote these values as $s_m$ and $s_n$ respectively. Again, we substitute $\lambda_k = \Lambda_m$, $u_k = u_i$ and $v_k = s_m u_i$ in Equation 10 and rearrange the terms to give us

$${}^uK_u + s_m\,{}^uK_v = {}^uD_u\Lambda_m + {}^uD_v s_m \Lambda_m. \quad (13)$$

Similarly, substituting $\lambda_k = \Lambda_n$, $u_k = u_j$ and $v_k = s_n u_j$ in Equation 10 yields

$${}^uK_u + s_n\,{}^uK_v = {}^uD_u\Lambda_n + {}^uD_v s_n \Lambda_n. \quad (14)$$

Now solving simultaneous Equations 13 and 14 assuming that ${}^uK_u$ and ${}^uK_v$ are the unknowns results in expressions

$$\begin{aligned} {}^uK_u &= \frac{{}^uD_u\,(s_n\Lambda_m - s_m\Lambda_n) + {}^uD_v s_m s_n\,(\Lambda_m - \Lambda_n)}{s_n - s_m}, \\ {}^uK_v &= \frac{{}^uD_u\,(\Lambda_n - \Lambda_m) + {}^uD_v\,(s_n\Lambda_n - s_m\Lambda_m)}{s_n - s_m}. \end{aligned} \quad (15)$$

Next, let us substitute $\lambda_k = \Lambda_m$, $u_k = u_i$ and $v_k = s_m u_i$ in Equation 11 and rearrange the terms. This results in

$$s_m\,{}^vK_v + {}^vK_u = {}^vD_v s_m \Lambda_m + {}^vD_u \Lambda_m \quad (16)$$

upon cancelling out the common nonzero factor $u_i$ from both sides. Similarly, by substituting $\lambda_k = \Lambda_n$, $u_k = u_j$ and $v_k = s_n u_j$ in Equation 11 we obtain

$$s_n\,{}^vK_v + {}^vK_u = {}^vD_v s_n \Lambda_n + {}^vD_u \Lambda_n. \quad (17)$$

Solving simultaneous Equations 16 and 17 for the unknowns ${}^vK_v$ and ${}^vK_u$ gives us the expressions,

$$\begin{aligned} {}^vK_v &= \frac{{}^vD_v\,(s_n\Lambda_n - s_m\Lambda_m) + {}^vD_u\,(\Lambda_n - \Lambda_m)}{s_n - s_m}, \\ {}^vK_u &= \frac{{}^vD_v s_m s_n\,(\Lambda_m - \Lambda_n) + {}^vD_u\,(s_n\Lambda_m - s_m\Lambda_n)}{s_n - s_m}. \end{aligned} \quad (18)$$

Next, we use Equations 15and 18 to derive the precondition ${}^{u}D_{u}{}^{v}D_{v} > {}^{u}D_{v}{}^{v}D_{u}$ (i.e. Equation 15 in the main paper) for linear stability at a mixed-mode bifurcation in absence of diffusion. For linear stability in absence of diffusion, one of the preconditions as given in Equation 11 states that ${}^{u}K_{u}{}^{v}K_{v} - {}^{u}K_{v}{}^{v}K_{u} > 0$. First, multiplying ${}^{u}K_{u}$ from Equation 15 with ${}^{v}K_{v}$ from Equation 18 results in

$$
\begin{aligned}
{}^{u}K_{u}{}^{v}K_{v} = & \frac{{}^{u}D_{u}\left(s_{n}\Lambda_{m} - s_{m}\Lambda_{n}\right) + {}^{u}D_{v}s_{m}s_{n}\left(\Lambda_{m} - \Lambda_{n}\right)}{s_{n} - s_{m}} \times \\
& \frac{{}^{v}D_{v}\left(s_{n}\Lambda_{n} - s_{m}\Lambda_{m}\right) + {}^{v}D_{u}\left(\Lambda_{n} - \Lambda_{m}\right)}{s_{n} - s_{m}}
\end{aligned}
$$

That is,

$$
\begin{aligned}
{}^{u}K_{u}{}^{v}K_{v}\left(s_{n} - s_{m}\right)^{2} = & \left({}^{u}D_{u}\left(s_{n}\Lambda_{m} - s_{m}\Lambda_{n}\right) + {}^{u}D_{v}s_{m}s_{n}\left(\Lambda_{m} - \Lambda_{n}\right)\right) \times \\
& \left({}^{v}D_{v}\left(s_{n}\Lambda_{n} - s_{m}\Lambda_{m}\right) + {}^{v}D_{u}\left(\Lambda_{n} - \Lambda_{m}\right)\right) \\
= & {}^{u}D_{u}{}^{v}D_{v}\left(s_{n}\Lambda_{m} - s_{m}\Lambda_{n}\right)\left(s_{n}\Lambda_{n} - s_{m}\Lambda_{m}\right) + \\
& {}^{u}D_{u}{}^{v}D_{u}\left(s_{n}\Lambda_{m} - s_{m}\Lambda_{n}\right)\left(\Lambda_{n} - \Lambda_{m}\right) + \\
& {}^{u}D_{v}{}^{v}D_{v}\,s_{m}s_{n}\left(\Lambda_{m} - \Lambda_{n}\right)\left(s_{n}\Lambda_{n} - s_{m}\Lambda_{m}\right) + \\
& {}^{u}D_{v}{}^{v}D_{u}\,s_{m}s_{n}\left(\Lambda_{m} - \Lambda_{n}\right)\left(\Lambda_{n} - \Lambda_{m}\right). \qquad (19)
\end{aligned}
$$

Similarly, multiplying ${}^{u}K_{v}$ from Equation 15 with ${}^{v}K_{u}$ from Equation 18 results in

$$
\begin{aligned}
{}^{u}K_{v}{}^{v}K_{u}\left(s_{n} - s_{m}\right)^{2} = & {}^{u}D_{u}{}^{v}D_{v}\,s_{m}s_{n}\left(\Lambda_{n} - \Lambda_{m}\right)\left(\Lambda_{m} - \Lambda_{n}\right) + \\
& {}^{u}D_{u}{}^{v}D_{u}\left(\Lambda_{n} - \Lambda_{m}\right)\left(s_{n}\Lambda_{m} - s_{m}\Lambda_{n}\right) + \\
& {}^{u}D_{v}{}^{v}D_{v}s_{m}s_{n}\left(s_{n}\Lambda_{n} - s_{m}\Lambda_{m}\right)\left(\Lambda_{m} - \Lambda_{n}\right) + \\
& {}^{u}D_{v}{}^{v}D_{u}\left(s_{n}\Lambda_{n} - s_{m}\Lambda_{m}\right)\left(s_{n}\Lambda_{m} - s_{m}\Lambda_{n}\right). \qquad (20)
\end{aligned}
$$

Now subtracting Equation 20 from Equation 19 gives us,

$$
\begin{aligned}
& \left({}^{u}K_{u}{}^{v}K_{v} - {}^{u}K_{v}{}^{v}K_{u}\right)\left(s_{n} - s_{m}\right)^{2} = \\
& \quad \left({}^{u}D_{u}{}^{v}D_{v} - {}^{u}D_{v}{}^{v}D_{u}\right)\left(s_{n}\Lambda_{m} - s_{m}\Lambda_{n}\right)\left(s_{n}\Lambda_{n} - s_{m}\Lambda_{m}\right) + \\
& \quad \left({}^{u}D_{u}{}^{v}D_{v} - {}^{u}D_{v}{}^{v}D_{u}\right)\,s_{m}s_{n}\left(\Lambda_{n} - \Lambda_{m}\right)^{2} \\
& \text{i.e. } \left({}^{u}K_{u}{}^{v}K_{v} - {}^{u}K_{v}{}^{v}K_{u}\right)\left(s_{n} - s_{m}\right)^{2} = \left({}^{u}D_{u}{}^{v}D_{v} - {}^{u}D_{v}{}^{v}D_{u}\right)\Lambda_{m}\Lambda_{n}\left(s_{n} - s_{m}\right)^{2}. \qquad (21)
\end{aligned}
$$

Assuming $s_{n} \neq s_{m}$, we factor out $\left(s_{n} - s_{m}\right)^{2}$ from both sides of Equation 21. This leaves us with

$$
{}^{u}K_{u}{}^{v}K_{v} - {}^{u}K_{v}{}^{v}K_{u} = \left({}^{u}D_{u}{}^{v}D_{v} - {}^{u}D_{v}{}^{v}D_{u}\right)\Lambda_{m}\Lambda_{n}. \qquad (22)
$$

For the boundary conditions discussed in Section D2, the LB operator $\nabla^{2}$ is *Hermitian* and all its eigenvalues such as $\Lambda_{m}$ and $\Lambda_{n}$ are non-negative. Thus, from Equation 22, the stability precondition ${}^{u}K_{u}{}^{v}K_{v} - {}^{u}K_{v}{}^{v}K_{u} > 0$ translates into

$$
{}^{u}D_{u}{}^{v}D_{v} > {}^{u}D_{v}{}^{v}D_{u}. \qquad (23)
$$

This is the same precondition as Equation 15 in the main paper.
