# Supplementary material for: Bifurcation Analysis of Reaction Diffusion Systems on Arbitrary Surfaces
Source: arXiv:1605.01583 ancillary file (2016-05-05)
Supplement: Supplementary file 2 [file SM02.pdf]

# Bifurcation Analysis of Reaction Diffusion Systems on Arbitrary Surfaces
# SM02: Framework Implementation Details and Additional Results

## A1 Implementation Details for Branch Tracing

The first task in branch tracing is to switch over to the new branch of patterns characterised by a given bifurcation pattern $\mathbf{x}_b = (\mathbf{u}_b, \mathbf{v}_b)$. While the linear stability analysis gives us $\mathbf{x}_b$, we are interested in a non-trivial solution $\mathbf{x}_s$ that fully satisfies the actual nonlinear PDE given in Equation 1 (Main Paper), near the bifurcation point $\mathbf{p}$ (with $\alpha = \alpha_0$) on the trivial branch. With $\mathbf{x}_h = (a_0, b_0)$ as the homogeneous solution at the bifurcation point $\mathbf{p}$, estimating a good starting point $\mathbf{x}_s$, with $\alpha \approx \alpha_0$, is a non-trivial task. The solution $\mathbf{x}_s$ must be qualitatively similar to $\mathbf{x}_b$ and yet far-enough away from the trivial branch to allow continuation along the new branch, without falling back to the trivial branch. We support three approaches to switch over to the new branch.

Our first approach is based on the *method of parallel computation* as suggested by Seydel (2010) (Section 5.6.3 in his book). Let us consider the FEM-discretised form of Equation 1 (Main Paper) expressed as

$$\mathbf{M}\frac{\partial \mathbf{x}}{\partial t} = \mathbf{f}(\mathbf{x}, \alpha). \tag{1}$$

Here, $\mathbf{x} = (a, b)$ is a vector representing the discretised and concatenated $a$ and $b$, and $\alpha$ is the continuation parameter. The *mass matrix* $\mathbf{M}$ and the vector $\mathbf{f}$ are obtained through an application of a *weak formulation* integration to Equation 1 (Main Paper) for a Galerkin method. In addition, $\partial\mathbf{x}/\partial t$ represents the discretisation of the temporal derivatives in Equation 1 (Main Paper).

Our aim is to find $\mathbf{x}_s$ and $\alpha$ near $\alpha_0$ such that $\mathbf{f}(\mathbf{x}_s, \alpha) = 0$ and $\mathbf{x}_s$ is near the bifurcation pattern $\mathbf{x}_b$, qualitatively. In a method of parallel computation, we achieve this by solving the following simultaneous equations,

$$\begin{bmatrix} \mathbf{f}(\mathbf{x}_h, \alpha) \\ \mathbf{f}(\mathbf{x}_s, \alpha) \\ \mathbf{x}_s(k) - \mathbf{x}_h(k) \end{bmatrix} = \begin{bmatrix} \mathbf{0} \\ \mathbf{0} \\ \varepsilon \end{bmatrix}. \tag{2}$$

Here, $\varepsilon$ is an arbitrary constant that fixes the distance between $\mathbf{x}_h$ and $\mathbf{x}_s$ along the $k$-th dimension of the solution space. Since we are on a trivial branch, $\mathbf{x}_h$ is known exactly for a given $\alpha$ and we only solve for the remaining two equations from the set, in our case. We solve the reduced set of equations using a *bordering algorithm* (Salinger et al, 2002) by iteratively computing

$$\begin{bmatrix} \mathbf{J}_{(\mathbf{x}_i,\alpha_i)} & \dfrac{\partial \mathbf{f}(\mathbf{x}_i,\alpha_i)}{\partial \alpha} \\ \mathbf{e}_k^T & \mathbf{0} \end{bmatrix} \begin{bmatrix} \Delta \mathbf{x}_i \\ \Delta \alpha_i \end{bmatrix} = \begin{bmatrix} -\mathbf{f}(\mathbf{x}_i,\alpha_i) \\ \varepsilon_i \end{bmatrix}, \tag{3}$$

$$\mathbf{x}_{i+1} = \mathbf{x}_i + \Delta \mathbf{x}_i, \quad i = 0,1,...$$

$$\alpha_{i+1} = \alpha_i + \Delta \alpha_i, \quad i = 0,1,...$$

until convergence on $\mathbf{f}(\mathbf{x}_i,\alpha_i) = 0$. Here, $\mathbf{J}$ is the Jacobian matrix for $\mathbf{f}$, $i$ the iteration count, and $\mathbf{e}_k$ a unit vector with all but the $k$-th element set to zero. We select $k$ such that it refers to the element in $\mathbf{x}_0$ that is expected to undergo maximum change in the first iteration while having at least half the magnitude of the largest element in $\mathbf{x}_0$. In other words $k$ satisfies the optimization $argmax_k\ |\Delta \mathbf{x}_0(k)|$, such that $|\mathbf{x}_0(k)| \geq ||\mathbf{x}_0||_\infty/2$. Initially, we set $\mathbf{x}_0 = \mathbf{x}_h + \varepsilon \mathbf{x}_b/||\mathbf{x}_b||_\infty$, $\alpha_0$ is available as the bifurcation point, and $\varepsilon_0 = \varepsilon\,(1 - \mathbf{x}_b(k)/||\mathbf{x}_b||_\infty)$. To simplify computations and aid convergence we set $\varepsilon_i = 0$, $\forall i > 0$. To avoid divergence, we further limit $\alpha_i$ by a positive, small constant $\alpha_\varepsilon$ such that $|\alpha_i - \alpha_0| < \alpha_\varepsilon$. Upon convergence, $||\mathbf{f}(\mathbf{x}_i,\alpha_i)||_2$ is less than a given error threshold and we set $\mathbf{x}_s = \mathbf{x}_i$.

Our second approach to branch switching is a simple modification of our first approach, and it is preferred for multiple and mixed-mode bifurcations. For such bifurcations, we may possibly compose infinite linear combinations of the basis eigenvectors $\mathbf{b}_k$ where each would give a valid solution near the bifurcation point $\alpha$. To avoid divergence into such possibilities we scale $\Delta \mathbf{x}_i$ with $w = |\widehat{\mathbf{x}}_b \cdot \widehat{\mathbf{x}}_i|^3$ at each iteration of the bordering algorithm. Here, $\widehat{\mathbf{x}}$ represents the unit vector along $\mathbf{x}$. Upon convergence, we set $\mathbf{x}_s = \mathbf{x}_i$. Finally, since an eigenvector is a dimensional characteristic and direction-agnostic, we repeat the above procedure with $-\mathbf{x}_b$ for branch switching and continuation thereafter.

On some rare occasions, the above switching methods may fail to converge, i.e, $||\mathbf{f}(\mathbf{x}_i,\alpha_i)||_2$ is greater than the given threshold. In such cases, our last approach sets $\mathbf{x}_s = \mathbf{x}_h + \varepsilon \mathbf{x}_b/||\mathbf{x}_b||_\infty$ with a small constant $\varepsilon$ and $\alpha = \alpha_0$. While this is a less reliable switching strategy it might still be possible to correct the initial bad $\mathbf{x}_s$ during branch continuation.

Once branch switching is accomplished, we follow the new branch by means of continuation. Our framework uses the *LOCA* and *NOX* packages from the Trilinos library to perform *pseudo arc-length continuation*. Continuation is performed for a fixed number of steps $i$. For the first continuation step, we start with $\mathbf{x} = \mathbf{x}_h$ as the current solution at $\alpha = \alpha_0$ and set $\mathbf{c}^0_{pred} = \mathbf{x}_s$ as the predicted new solution at $\alpha_{step(0)} = \alpha_0 + \Delta step(0)$. Here $\Delta step(i)$ is the step size for step $i$. For all subsequent steps we use a *secant method* to predict $\mathbf{c}^i_{pred}$ as the new solution at $\alpha_{step(i)} = \alpha_{step(i-1)} + \Delta step(i)$. Each predicted solution $\mathbf{c}^i_{pred}$ is corrected to $\mathbf{c}^i$ for

$\mathbf{f}(\mathbf{c}^i, \alpha_{step(i)}) = 0$ using a *line search based* iterative method from the nonlinear solver NOX. We initialize the NOX solver with the predicted solution as $\mathbf{c}^i_0 = \mathbf{c}^i_{pred}$. For each iteration $j$ of the NOX solver, with $\mathbf{c}^i_j$ as the current solution, we compute a direction vector $\mathbf{d}$, and use a *Newton method* to solve the linear system $\mathbf{J}_{\mathbf{c}^i_j, \alpha_{step(i)}} \mathbf{d} = -\mathbf{f}(\mathbf{c}^i_j, \alpha_{step(i)})$. Since our Jacobian matrix $\mathbf{J}$ is not Hermitian, we use the *biconjugate gradient method* as implemented in the AztecOO package to solve the above linear system. Another alternative is to use a *generalized minimal residual method* for robustness, however, we found it to be too slow for the trade-off, in general. In order to improve the convergence characteristics of the linear solver, we use a default preconditioner as implemented in the *IFPACK* package from the Trilinos library. At the end of each nonlinear solver iteration, the solution is updated as $\mathbf{c}^i_{j+1} = \mathbf{c}^i_j + \mathbf{d}$. Upon convergence for the nonlinear solver, the new solution on the branch $\mathbf{c}^i = \mathbf{c}^i_j$ is output along with $\alpha_{step(i)}$ and used for the next continuation step.

We use an adaptive approach for continuation. The step size $\Delta step(i)$ is scaled-up upon successful convergence of a solution $\mathbf{c}^i$. Similarly, upon a failure of the nonlinear solver $\Delta step(i)$ is scaled-down, for a repeat attempt. To avoid stagnations or branch-jumps $\Delta step(i)$ is bounded, i.e. $(step_{\min} \leq \Delta step(i) \leq step_{\max})$. Furthermore, there are global limits on $\alpha$ as $\alpha_{\min} \leq \alpha \leq \alpha_{\max}$. Finally, in order to improve the smoothness of current branch tracing we impose a *tangent scale factor* to manoeuvre the direction of the *continuation curve* in conformance with the tangents to the curve at two previous solution points. Branch direction is of greater importance for tracing at its origin. We thus, optionally, initialise the tracer with $\mathbf{x} = \mathbf{x}_s$ as the current solution while setting $\mathbf{c}^0_{pred} = \mathbf{x}_h - (\mathbf{x}_s - \mathbf{x}_h)$. Such a predicted $\mathbf{c}^0_{pred}$ is usually not converged and an additional initial correction step by the tracer helps to better profile the branch curvature near its origin. These features are supported by LOCA and explained in detail in its documentation.

## A2 Framework Configurability

Section 4 in the main paper provides implementation details for our framework. We intend to share the code for our framework in public domain and here we document its configurability for various operations that it may perform independently.

Our framework is flexible and easily configurable to use either of the *proposed* and *reference* methods discussed in Section 4 for the main paper. Furthermore, our framework is easily parallelisable for the proposed method as it allows independent execution of one or more operations. We discuss operation-specific configurable aspects of the framework below. In order to use our framework for a specific RD system, it needs to be adapted. Again, we explain these adaptations in respective subsections for corresponding operations.

## A2.1 Computing Eigenvectors of the Laplace-Beltrami Operator

Section 4.1 in the main paper explains how we numerically approximate the eigenfunctions of the Laplace-Beltrami operator $\nabla^2$ operating on an arbitrary surface domain $\Omega$ with FEM discretised eigenvectors $\mathbf{b}_k$. Our framework reads in a given mesh file (in .MSH file format) which contains the definition of the arbitrary domain $\Omega$. It then constructs the *stiffness* and *mass* matrices $\mathbf{K}$ and $\mathbf{M}$ in Equation 18 (Main Paper) using the Deal.II library and solves the general eigenvalue problem in Equation 18 (Main Paper) to compute eigenvectors $\mathbf{b}_k$ using the Trilinos library. The user can configure our framework to choose: (i) the order of the FEM (upto 3), (ii) the number of eigenvectors to be computed, and (iii) a shift factor in the eigenspectrum for the *shift-invert* approach. The resultant set $\mathbf{S_b} = \{\mathbf{b}_k\}$ of eigenvectors is output and stored into a file along with corresponding eigenvalues, $\mathbf{S}_\Lambda = \{\lambda_k\}$. For the simplest of applications concerned with the profile of simple bifurcation patterns near homogeneity, it suffices to solve for $\mathbf{S_b}$ alone. For more advanced applications additional operations can be performed using $\mathbf{S_b}$ and $\mathbf{S}_\Lambda$.

## A2.2 Computing Bifurcation Points and Patterns

Section 4.2 in the main paper explains how sets $\mathbf{S_b} = \{\mathbf{b}_k\}$ and $\mathbf{S}_\Lambda = \{\lambda_k\}$ are used to construct bifurcation patterns and compute their respective bifurcation points. For this operation, the user provides previously computed sets $\mathbf{S_b}$ and $\mathbf{S}_\Lambda$ to the framework as inputs. The user also provides the values for all known control parameters in set $\mathbf{p}$ (Refer to 4.2 in the main paper for details of $\mathbf{p}$). There are three possibilities for a type of bifurcation, i.e. a *simple, multiple or mixed-mode* bifurcation. The user specifies the type of bifurcation and also if it is *exclusive* or not, in the case of simple and multiple bifurcations. In addition, for simple bifurcations, the user inputs a *job-list* of indices $\{i\}$, each representing a potential pattern. For multiple bifurcations, the user provides a similar job-list with each entry consisting of: (a) a nested list of indices $\{i\}$, and (b) a nested list of weights $\{u_i\}$ for linear combination of eigenvectors, $\mathbf{b}_i$. For a mixed mode bifurcation case, the user provides a job-list where each entry consists of: (a) two nested lists of indices $\{i\}$ and $\{j\}$, and (b) two lists of weights $\{u_i\}$, and $\{u_j\}$. For all three cases, our framework outputs one vector $\mathbf{x}_b = (\mathbf{u}_b, \mathbf{v}_b)$ as the bifurcation pattern* along with corresponding bifurcation location $\mathbf{p}$ for each entry in the job-list.

## A2.3 Configuring Branch Tracing

Section 4.5 in the main paper explains how our framework performs branch tracing. We need to first adapt the framework to perform branch switching and tracing for a given specific RD system. In particular, we need an RD system specific implementation to compute:

*computed as explained in Section 4 in the main paper.

- $\mathbf{f}$: The $\mathbf{f}$-vector from Equation 1, representing the temporal derivatives in the partial differential equations, under a *weak formulation*.
- $\mathbf{J}$: Jacobian matrix for the $\mathbf{f}$-vector.
- $\partial \mathbf{f}/\partial \alpha$: Partial derivative of the $\mathbf{f}$-vector w.r.to the continuation parameter $\alpha$.

As a first step in implementing these routines, the user has to apply a weak Galerkin method to formulate $\mathbf{f}$, $\mathbf{J}$ and $\partial \mathbf{f}/\partial \alpha$ in terms of FEM-shape functions, their gradients, vector $\mathbf{x}^{\dagger}$ and system parameters $\mathbf{p}$. With the required FEM-based formulae defined, as the next step, the user need to implement routines for approximating surface integrals by applying a *Gauss quadrature rule* to approximate those integrals with cumulative weighted summations over all finite elements. These implementations are made easy with the *application programming interface (API)* for the Deal.II library (Bangerth et al, 2007). Our framework provides generic classes to be extended through inheritance to facilitate user-defined implementations using the Deal.II and Trilinos (Heroux et al, 2005) libraries. For performing branch tracing, the user provides a job-list with each entry containing: (a) a previously computed bifurcation pattern $\mathbf{x}_b$, (b) known parameter values $\mathbf{p} - \{\alpha\}$, and (c) a previously computed continuation parameter value $\alpha$ at the corresponding bifurcation point. In addition, the user provides the triangulation mesh file in *MSH* format for the surface definition, i.e., $\Omega$, same as in the case of eigenvector computation operation. Also, the user can configure the framework to: (a) select the branch switching strategy with or without *cos factor scaling* (see Section 4.5 in the main paper), (b) the pattern scale $\varepsilon$ as given in Equation 2, (c) $\alpha_{\min}$, $\alpha_{\max}$, $step_{\min}$, $step_{\max}$, (d) a flag to use branch guidance at its origin (see last paragraph in Section 4.5 in the main paper), (e) a flag to use *tangent scale factor* and (f) an error limit for solution convergence. The framework then loads the input data, traces a branch for each entry in the job-list and outputs the resulting solutions along with respective $\alpha$ values in a separate file.

## A3 Quantitative Evaluation with Murray's model

In this section we provide additional numerical results for quantitative evaluation of our framework with Murray's model. Please refer to Section 6.2 in the main paper for the experimental setup details and our methodology for computing the *root mean square error*, i.e. $\varepsilon_{RMS}$ for an emergent pattern under consideration.

Figure 1 plots RMS errors $\varepsilon_{RMS}$ in computing 100 emergent patterns with our proposed method and the reference method, on a *log-lin* semilog scale. We assign each emergent pattern an index based on its nearest eigenvector $\mathbf{b}_i$ corresponding to eigenfunction $\phi_i$ for the Laplace-Beltrami operator. We use the same quasi grid‡ with about 4400 nodes with an FEM first order discretisation for both, our proposed and the reference method. We solve for the eigenvectors with convergence limit set

† representing a potential (discretised) solution to the RD system under consideration.

‡ See Figure 4a for an example of a quasi grid triangulation.

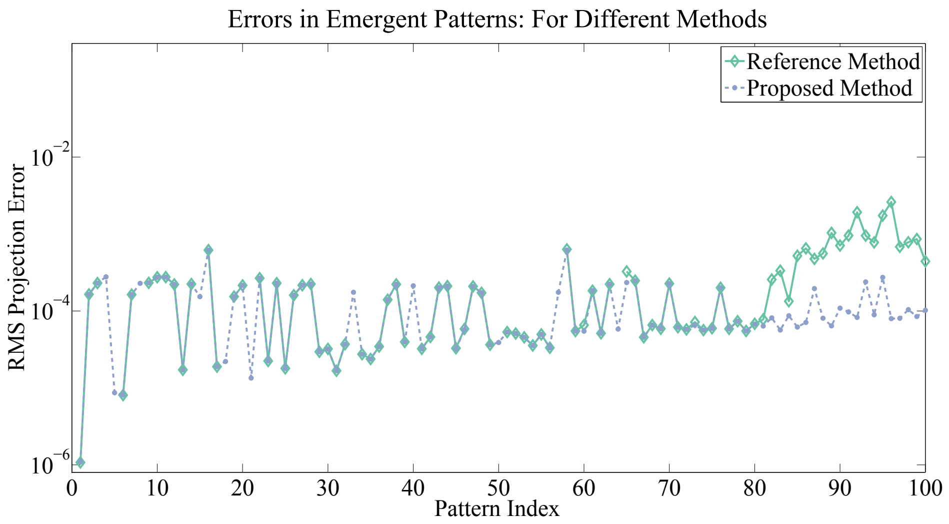


Figure 1: RMS errors for different methods in computing 100 emergent patterns for Murray's model acting on a rectangular domain $\Omega$.

in the order of $10^{-12}$ and this results in low RMS errors in general, on a relative scale of $10^{-4}$ to $10^{-6}$. Visually, the emergent patterns $\mathbf{u}_b$ and their projections $\widehat{\mathbf{u}_b}$ look indistinguishable for our proposed method. In conclusion, the accuracy of our proposed direct approach is comparable to that of the reference method and even better for the emergent patterns corresponding to higher eigenvalues. Also, importantly, while the reference method misses out on some emergent patterns[§] due to multiple bifurcations or failures of the chosen test function, our proposed method discovers all emergent patterns.

Next, we analyse the impact of FEM order on the accuracy of our proposed method. We use a regular mesh as shown in Figure 4a for FEM discretisations of order 1, 2 and 3 with about 4400 nodes in each case[¶]. Figure 2 shows that for FEM order 1, the relative error in locating a bifurcation point is $< 2\%$ but it grows with the magnitude of the corresponding eigenvalue. As expected in this case, using a higher order FEM improves the accuracy in locating bifurcation point considerably. However, Figure 3 shows that the accuracy in computing emergent patterns generally remains the same or even decreases with the use of higher order FEMs. Apparently, at a given resolution, the size of the finite element is important and the very high accuracy in computing eigenvalues (and thus the bifurcation points) is achieved with higher order FEMs at the expense of relatively, slightly inaccurate eigenvectors. Here we note that the relative errors for the first order FEM reduces significantly with mesh resolution (not shown) as in the case of the Brusselator model (see Figure 4 in the main paper).

[§]indicated by discontinuities in the graph for RMS errors for the reference method in Figure 1.
[¶]This implies that for a higher order FEM, we use comparatively fewer finite elements.

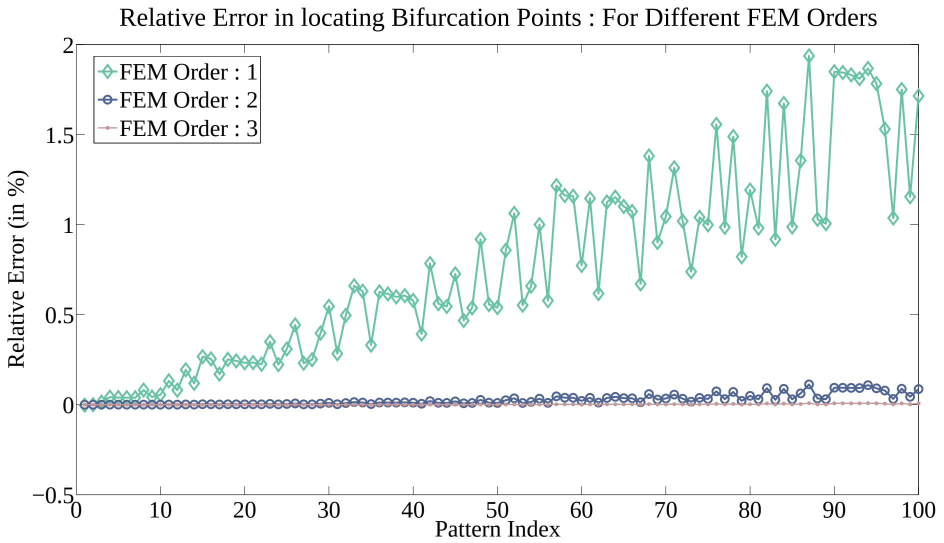


Figure 2: Relative error in computing bifurcation point locations for 100 emergent patterns for our proposed method with different FEM orders.

We also study the influence of mesh triangulation on error statistics using three different FEM triangulations of order one with about 4400 nodes. We use: (a) a perfect rectilinear mesh with *regular grid* of quad elements, (b) a *quasi grid* similar to the regular grid with slight, random perturbations to the interior nodes, and (c) a *random uniform* mesh with arbitrary elements of about equal size; see Figure 4a. Figure4b show the errors in computing emergent patterns for these different triangulation schemes. Clearly, with a *regular grid*, computed emergent patterns have a significantly high numerical accuracy (RMS errors are on the order of $10^{-5}$ to $10^{-10}$ on a relative scale). Even with slight perturbations as in the case of *quasi grid*, the numerical accuracy reduces by few orders of magnitude (RMS errors are on the order of $10^{-4}$ to $10^{-5}$ in general). For an arbitrary *random uniform* triangulation, the accuracy drops slightly with RMS errors on the order of $10^{-4}$. Here we note again that all eigenvectors are resolved with a convergence limit on the order of $10^{-12}$ and all emergent patterns appear to be good qualitatively. Also, as noted earlier with the Brusselator model, numerical accuracy increases with mesh resolution (not shown). Thus, a regular grid triangulation is warranted for applications with low resolution meshes and a high expected numerical accuracy for computed patterns.

## References

Bangerth W, Hartmann R, Kanschat G (2007) deal.II – a general purpose object oriented finite element library. ACM Trans Math Softw 33(4):24/1–24/27

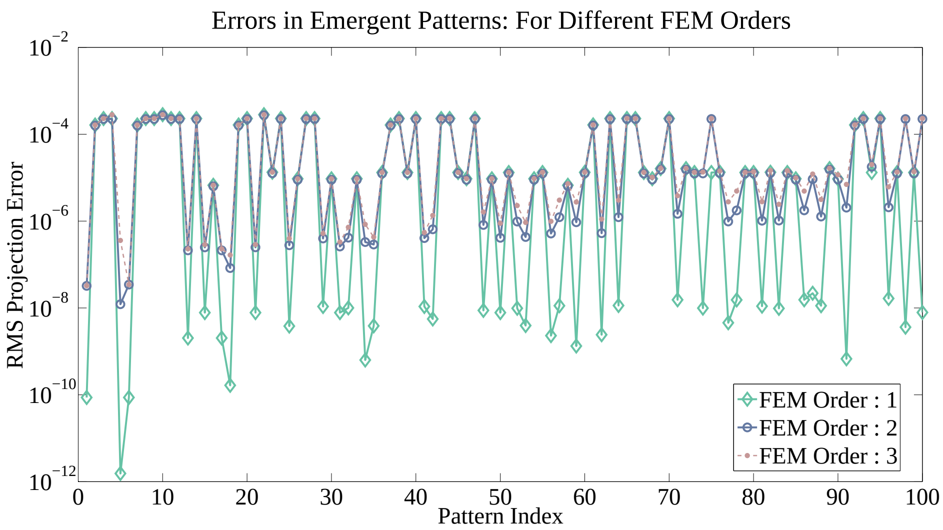


Figure 3: RMS error in computing 100 emergent patterns for our proposed method with different FEM orders.


Heroux MA, Bartlett RA, Howle VE, Hoekstra RJ, Hu JJ, Kolda TG, Lehoucq RB, Long KR, Pawlowski RP, Phipps ET, et al (2005) An overview of the trilinos project. ACM Transactions on Mathematical Software (TOMS) 31(3):397–423

Salinger AG, Bou-Rabee NM, Pawlowski RP, Wilkes ED, Burroughs EA, Lehoucq RB, Romero LA (2002) Loca 1.0 library of continuation algorithms: theory and implementation manual. Sandia National Laboratories, Albuquerque, NM, Technical Report No SAND2002-0396

Seydel R (2010) Practical bifurcation and stability analysis. Springer

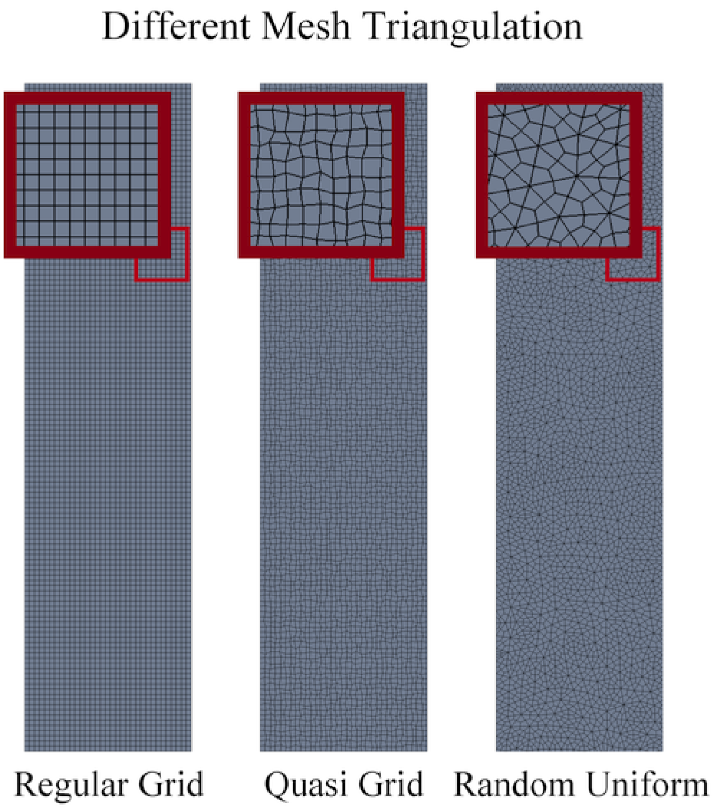


(a) Different FEM Mesh Triangulation.

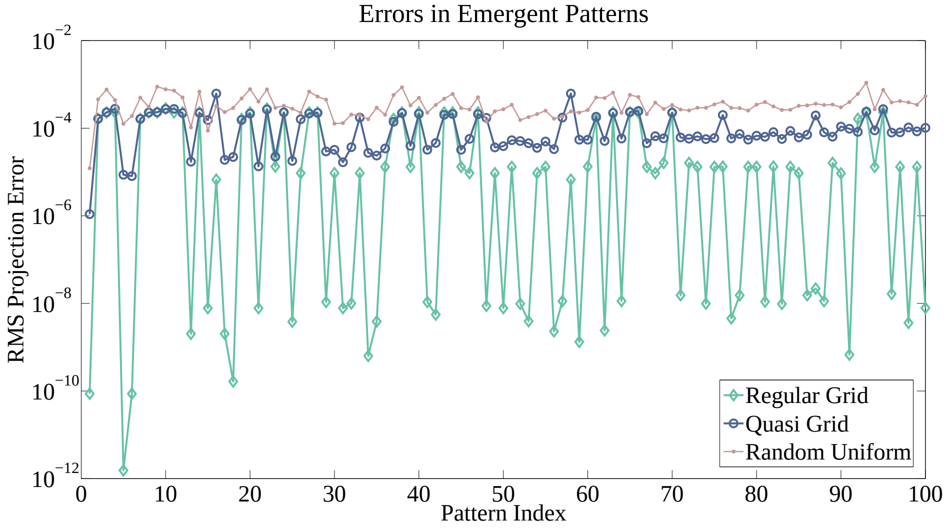


(b) Error plots.

Figure 4: RMS errors in computing 100 emergent patterns using our proposed method with different mesh triangulation for Murray's model.
